# Supplementary material for: AdaDiff: Accelerating Diffusion Models through Step-Wise Adaptive Computation
Source: arXiv:2309.17074 source file (2024-08-16)
Supplement: Supplementary file 1 [file appendix.tex]

\clearpage
\section{Appendix}
\subsection{More Experimental Setup}
\noindent \textbf{Dataset \& Baseline.} CIFAR-10 \cite{krizhevsky2009learning}, Celeb-A \cite{liu2015faceattributes} are used to evaluate our methods and other methods on unconditional generation. CIFAR-10 is a small-size dataset with a resolution of 32$\times$32. The Celeb-A
dataset, which includes 162,770 human faces, is a widely used dataset for unconditional image generation with a resolution of 64$\times$64. ImageNet~\cite{deng2009imagenet} is a large-scale dataset with 1000 classes, which is used to evaluate class-conditional generation. Text-guided generation is evaluated on MS-COCO~\cite{lin2014microsoft} dataset. MS-COCO consists of 5 image captions for every image and contains 82,783 training images and 40,504 validation images. The resolution of ImageNet and COCO is both 256$\times$256.
We compare our method with existing early exiting methods, BERTxiT~\cite{xin2021berxit} and CALM~\cite{schuster2022confident}. Since BERTxiT and CALM are originally implemented on language models, we re-implement these methods on diffusion models. BERTxiT utilizes a learning strategy to extend early exiting to BERT models and apply average layer-wise loss ($L$ = $\frac{1}{N} \sum_{i=1}^N L_i$, N is the number of layers) to train the network while CALM apply decay layer-wise loss ($L$ = $\frac{i}{N} \sum_{i=1}^N L_i$). Furthermore, CALM uses the similarity of adjacent layers and confidence to decide to exit and calibrates local early exits from global constraints. In our experiments, we follow their training strategy and we only apply similarity to decide exiting for CALM since confidence-based exiting is hard to be applied to diffusion models. During training, we choose the best epoch of BERTxiT and CALM for a fair comparison.

\textbf{Implementation Details.} On ImageNet 256$\times$256, we utilize the U-ViT-Large model with 21 layers and 16 attention heads while it is the U-ViT-Small model with 13 layers and 8 attention heads on other datasets. The hidden size of the network is 512 and 1024 for small and large models. We use a weight decay strategy and apply a weight decay of 0.03 for all datasets. We try the running coefficients $\beta_1, \beta_2$ of AdamW among {0.9, 0.99, 0.999}, and find that ($\beta_1, \beta_2$ ) = (0.99, 0.99) performs well for all datasets. On ImageNet 256$\times$256, ImageNet 512$\times$512 and MS-COCO, we adopt classifier-free guidance~\cite{ho2022classifier} following~
 \cite{rombach2022high}. We follow latent diffusion models ~\cite{rombach2022high} for high-resolution image generation. Specifically, for images at 256$\times$256 resolutions, we first convert the input images to latent representations at 32×32 resolutions, using the pre-trained image autoencoder provided by Stable Diffusion~\cite{rombach2022high}. All experiments are conducted on 4 A6000.

\subsection{More Experimental Results}
\subsubsection{Statistics of Exited Layers.}
We provide more experimental analysis about our proposed dynamic early exiting strategy. We report the average exited layer ratio of our model with different thresholds on the CIFAR-10 dataset, as shown in Figure~\ref{Fig:layer}. In the left figure, the experiment is conducted with a relatively low uncertainty threshold. Most computations are fully operated while there are still some parts of computation that are early stopped. In contrast, with a higher uncertainty threshold, most of the computations are terminated at the beginning which means some easy samples are allocated with less computation. This shows that with threshold control, our estimated uncertainty achieves a good trade-off between quality and efficiency.
\begin{figure*}[t]
\begin{center}
\subfloat[]{\includegraphics[width=0.4\textwidth]{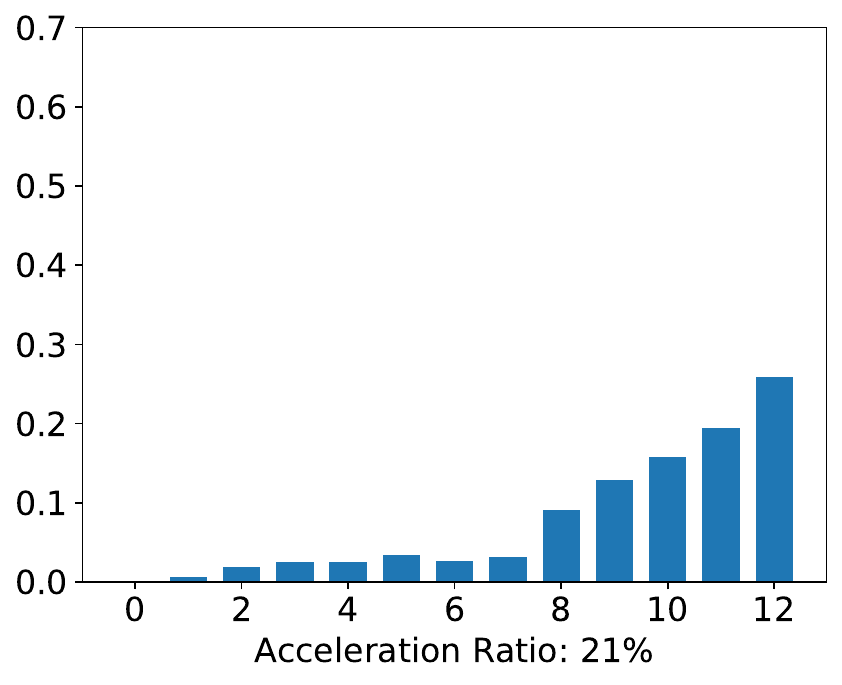}}
\subfloat[]{\includegraphics[width=0.4\textwidth]{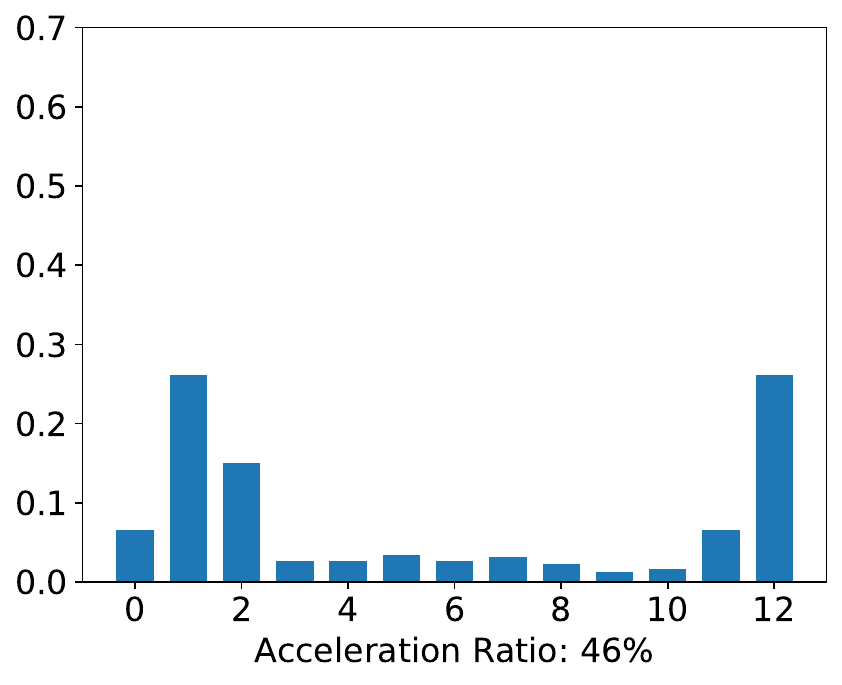}}
\end{center}
\caption{Statistics of exited layers on CIFAR-10. The horizontal axis represents the number of layers used for computation. The vertical axis refers to the ratio of the number of steps that utilize specific layers to the number of total sampling steps. We compute the average ratio across the whole dataset.}
\label{Fig:layer}
\end{figure*}

\subsubsection{Results on CNN-based Models.}
\begin{table}[t]
    \centering
    \caption{The performance and efficiency of AdaDiff on CNN-based models. Our method obtains similar performance with a high acceleration ratio as Transformer-based models, showing the compatibility of our approach with the two structures. }
    \vspace{-4mm}
    \begin{tabular*}{8cm}{c|cc|cc}
    \hline
    \hline
         \multirow{2}*{Methods} & \multicolumn{2}{c|}{CIFAR-10} &\multicolumn{2}{c}{CelebA} \\
         & FID  & Layers Ratio  & FID  & Layers Ratio  \\
    \hline
       DDIM (50 steps) &4.67 & 1  &9.17 & 1  \\
       Ours (50 steps) &5.43 & -37.4\%  &10.34 & -39.8\%  \\
    \hline
    \hline
    DDIM (100 steps) &4.16 & 1  &6.53 & 1  \\
    Ours (100 steps) &4.98 & -40.8\%  &7.35 & -41.5\%  \\
       % &Ours &\textbf{8.9} & \textbf{-40.8\%}   \\
    \hline
    \hline
    \end{tabular*}
    
    \label{tab:cnn}
\end{table}

Our method can be plugged into any framework easily such as Transformer and CNN. Therefore, we also provide the results on CNN-based models such as DDIM as shown in Table~\ref{tab:cnn}. The backbone of DDIM applies the UNet structure, which consists of resolution upsampling and downsampling. To ensure resolution consistency, we force the output of each layer to be the same resolution by interpolation. We utilize the open-source code from the official repository and conduct a group of experiments on several datasets. Our experiments are conducted with different sampling steps, 50 and 100 steps.
On CelebA and CIFAR-10, our AdaDiff is able to achieve around 40\% layer reduction ratio with a slight performance drop. 
\subsubsection{Results and Discussions on Different Sampling Strategies.}
In this section, we first provide more experimental results on our methods with different sampling strategies to show compatibility with other acceleration methods. Based on the results, we start an insightful discussion about the experimental observation and provide some assumptions for the results, which are left for future work to validate.

The results are shown in Table~\ref{tab:sampling}. There are several conclusions drawn from the results:

\textbf{The training of AdaDiff brings extra performance benefits.} Besides using DPM-Solver on CIFAR-10 datasets, our AdaDiff achieves better FID performance compared with baseline models. More specifically, utilizing the EM sampling strategy with 1000 steps, U-ViT achieves 3.11 and 2.87 FID on CIFAR-10 and CelebA, respectively. Without acceleration via early exiting, AdaDiff obtains 2.7 and 2.63 FID on each dataset. With 50 sampling steps by DPM-solver strategy on CelebA, our method achieves surprisingly 1.8 FID while U-ViT only gains 3.3 FID, bringing more than 45\% performance improvement.

\textbf{AdaDiff is compatible with other acceleration methods.}  As shown in Table~\ref{tab:sampling}, AdaDiff is able to be combined with other acceleration methods. The performance stays consistent with the combination of other methods. More concretely, utilizing the Euler Maruyama sampling strategy, AdaDiff achieves 3.7 and 3.9 FID with 47.7\% and 46.2\% layer reduction on CIFAR-10 and CelebA respectively. Furthermore, for the DPM-Solver with 50 sampling steps, AdaDiff also obtains 6.9 and 3.7 FID on each dataset while the performance of baselines is 4.5 and 3.3 respectively.

\textbf{Discussion.} A natural question for the results in Table~\ref{tab:sampling} is why the FID value of AdaDiff with DPM-solver is better than AdaDiff with Euler Maruyama. We believe the reason is the existence of model overfitting in pre-trained weights. With our UA-Loss, different training steps contribute unequally to model fitting, which potentially prevents the model from being overfitting. For future works, this could be a potential way to reduce the possibility for models to be overfitting.

\begin{table*}[t]
 % \addtolength{\tabcolsep}{0.5pt}
 
 \caption{More results of different sampling strategies on CIFAR-10 and Celeb-A datasets. EM: Euler Maruyama sampling with 1000 steps. DPM: DPM-solver with 50 steps.}
    \centering
    \begin{tabular*}{8.5cm}{lccccc}
    \toprule
    \toprule
        \multirow{2}*{Methods} & 
        \multicolumn{2}{c}{CIFAR-10 32$\times$32} & &
        \multicolumn{2}{c}{CelebA 64$\times$64}\\
        \cmidrule{2-3}
        \cmidrule{5-6}
         & FID  & Layers Ratio  & & FID & Layers Ratio  \\
    \midrule
       U-ViT + EM &3.11 & 1  &  &2.87 & 1    \\
    % \cline{2-8}
     % \hline
       U-ViT + DPM &4.5 &1  &  &3.3 &1    \\
       \hline
       Ours + EM w/o EE &2.7 &1 & &2.63 & 1     \\
      Ours + DPM w/o EE &5.2 &1  & &1.8 &1     \\
      \hline
      Ours + EM &3.7 &-47.7\% & &3.9 & -46.2\% \\
      Ours + DPM &6.9 &-43.1\% & &3.7 & -41.3\% \\
    % \cline{2-8}
     \midrule
     \bottomrule
    \end{tabular*}
    \label{tab:sampling}
\end{table*}

\subsection{Error Curve Comparison}
\begin{figure}[h]
\begin{center}
\subfloat[CIFAR-10]{\includegraphics[width=0.24\textwidth]{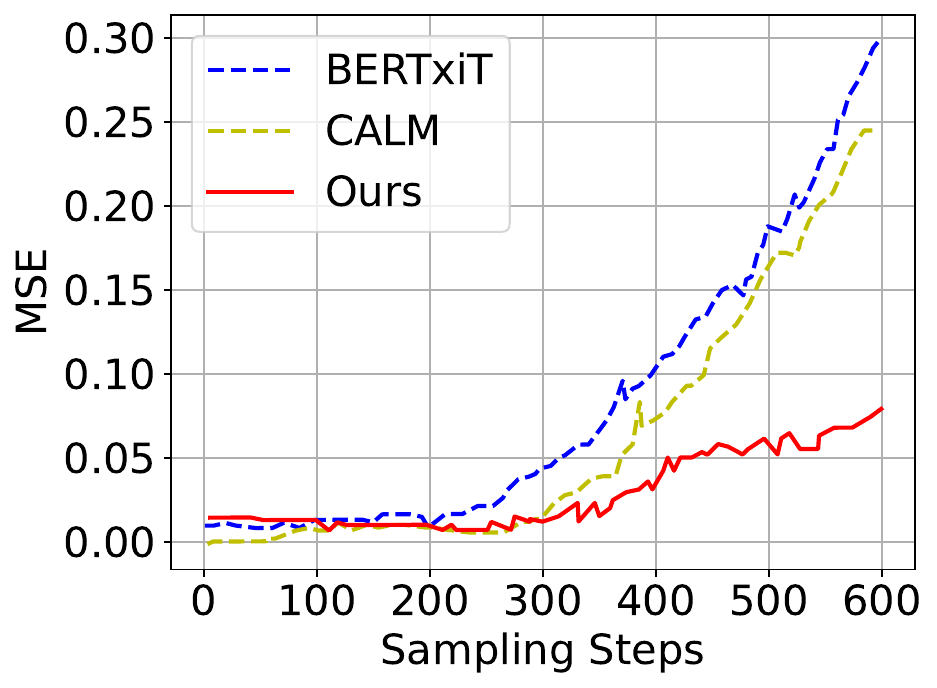}}
\subfloat[Celeb-A]{\includegraphics[width=0.24\textwidth]{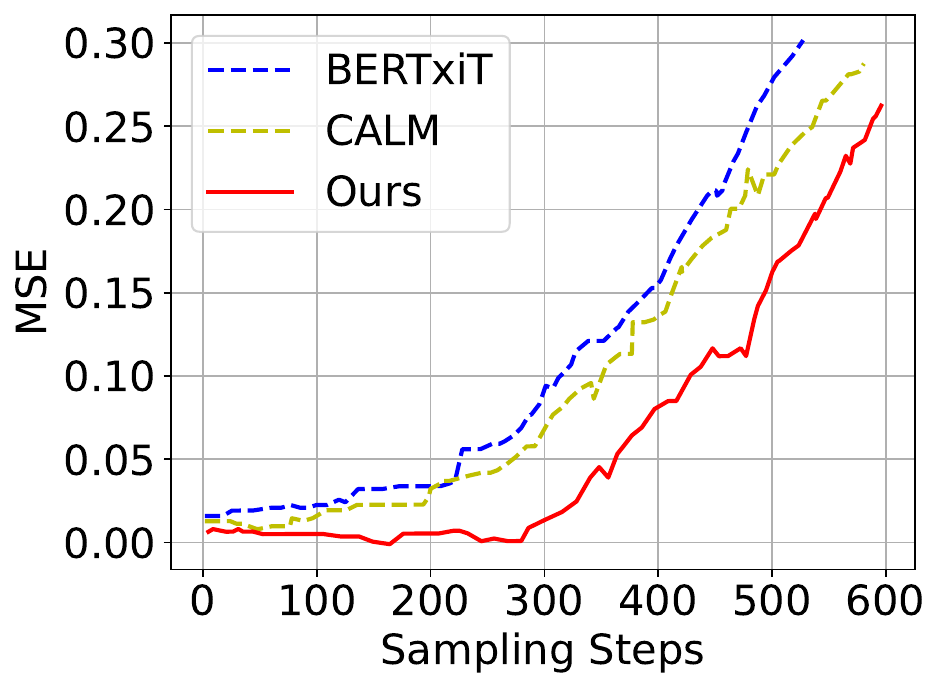}}
\subfloat[ImageNet]{\includegraphics[width=0.24\textwidth]{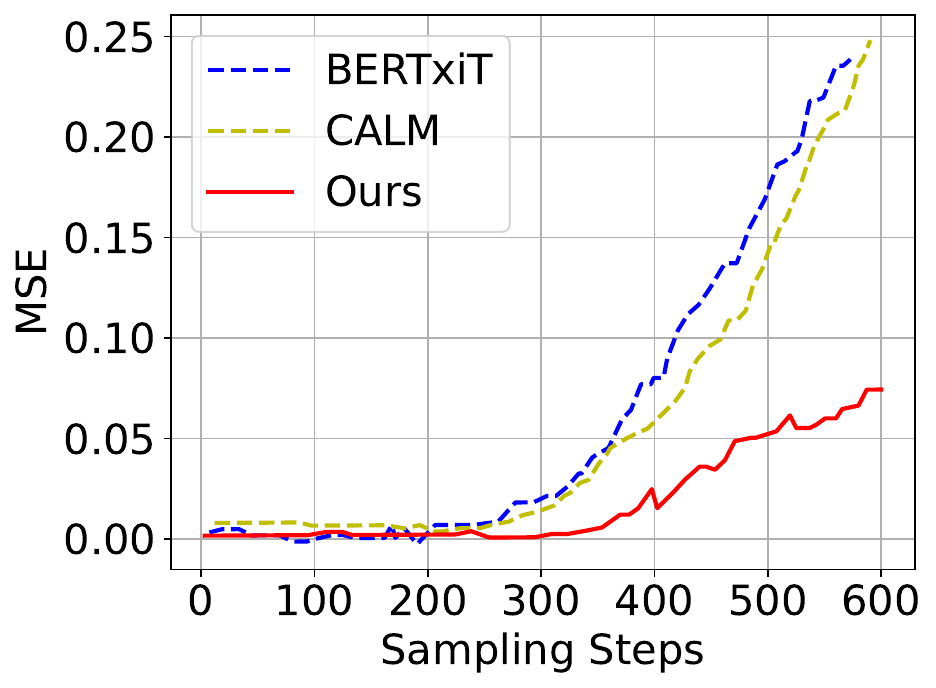}}
\subfloat[MS-COCO]{\includegraphics[width=0.24\textwidth]{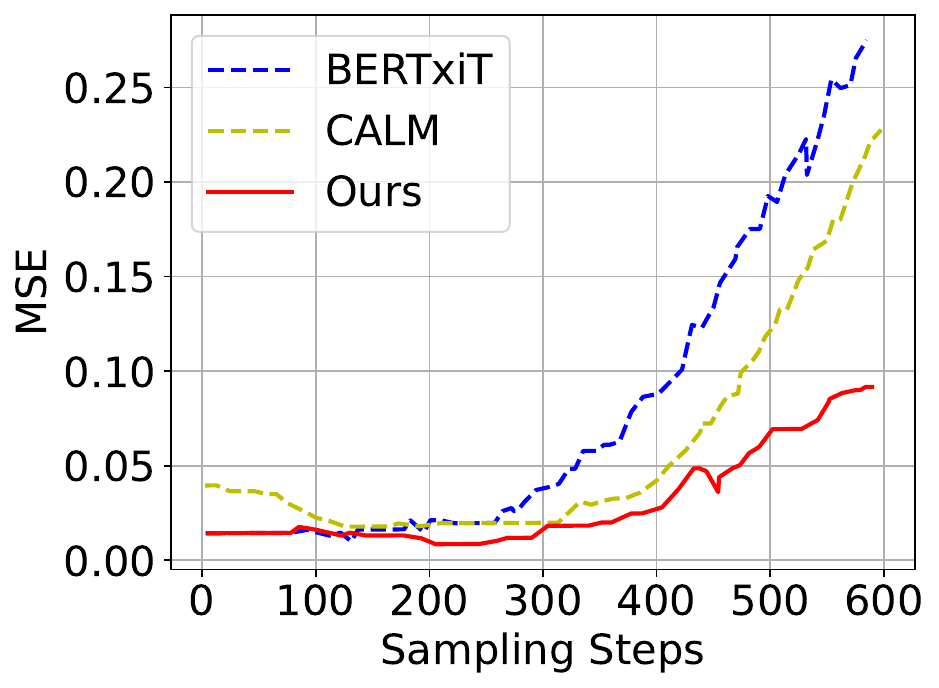}}
\end{center}
\caption{Error curve comparison of DeeDiff and other early exiting methods on CIFAR-10, Celeb-A, ImageNet and COCO.}
\label{Fig:err}
\end{figure}
Besides uncertainty map visualization, we show the error accumulation curve of different methods in comparison with the baseline on several datasets, as shown in Figure~\ref{Fig:err}. With early exited layers, the error of BERTxiT and CALM starts to increase as the number of sampling steps increments. The error curve of our method is always below that of other methods, which means that despite skipping many layers, the error accumulation of our method is still smaller than that of other methods.
This proves that our proposed uncertainty-aware layer-wise loss is able to benefit the whole generation timesteps and thus incurs lower error accumulation.

\subsection{More Samples Results}
More generation samples can be found in Figure~\ref{fig:enter-label}.
\begin{figure*}[ht]
    \centering
    \subfloat[CIFAR-10]{\includegraphics[width=0.45\textwidth]{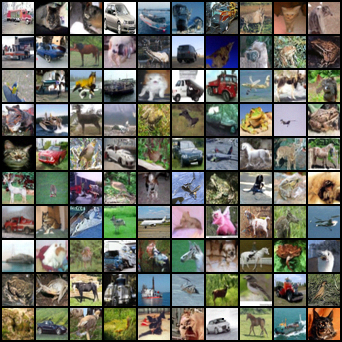}}
    \hspace{0.5cm}
    \subfloat[Celeb-A]{\includegraphics[width=0.45\textwidth]{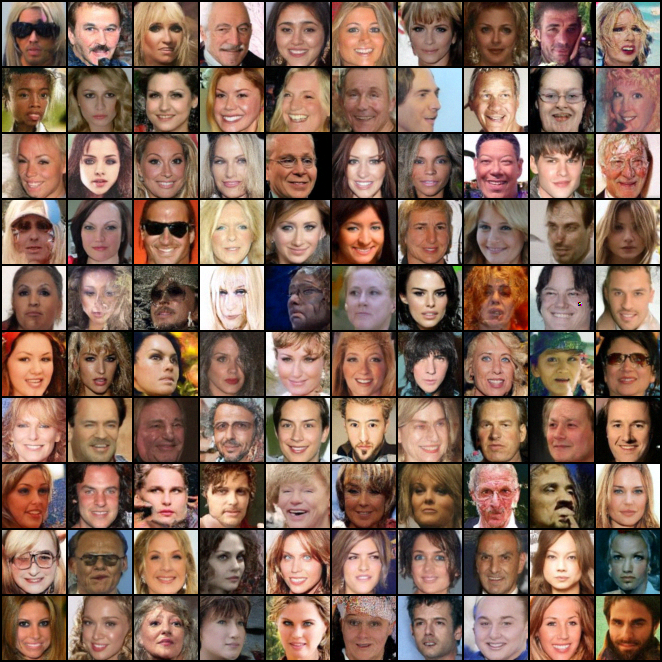}}
    
    \subfloat[MS-COCO]{\includegraphics[width=0.5\textwidth]{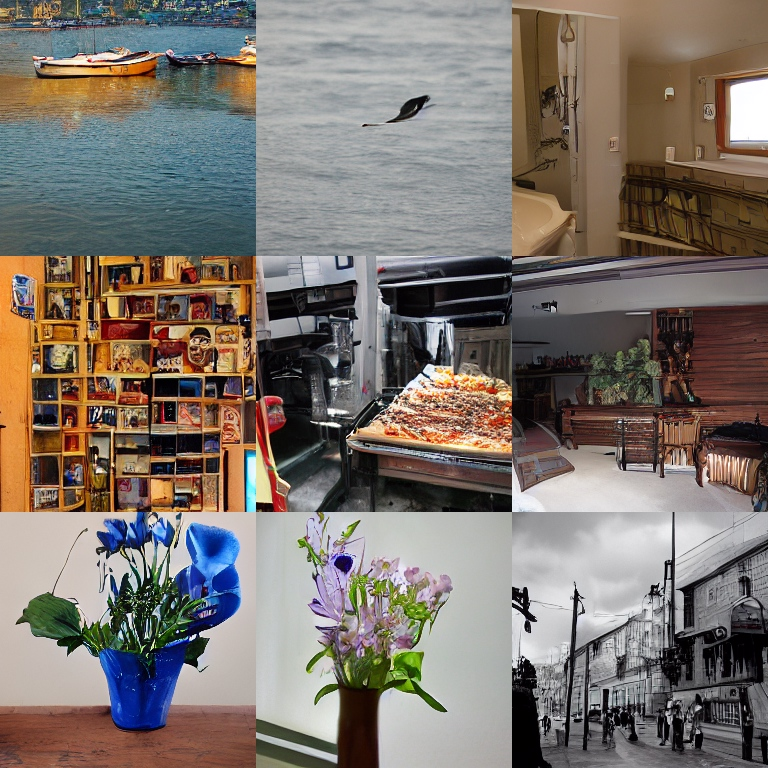}}
    
    \subfloat[ImageNet]{\includegraphics[width=1\textwidth]{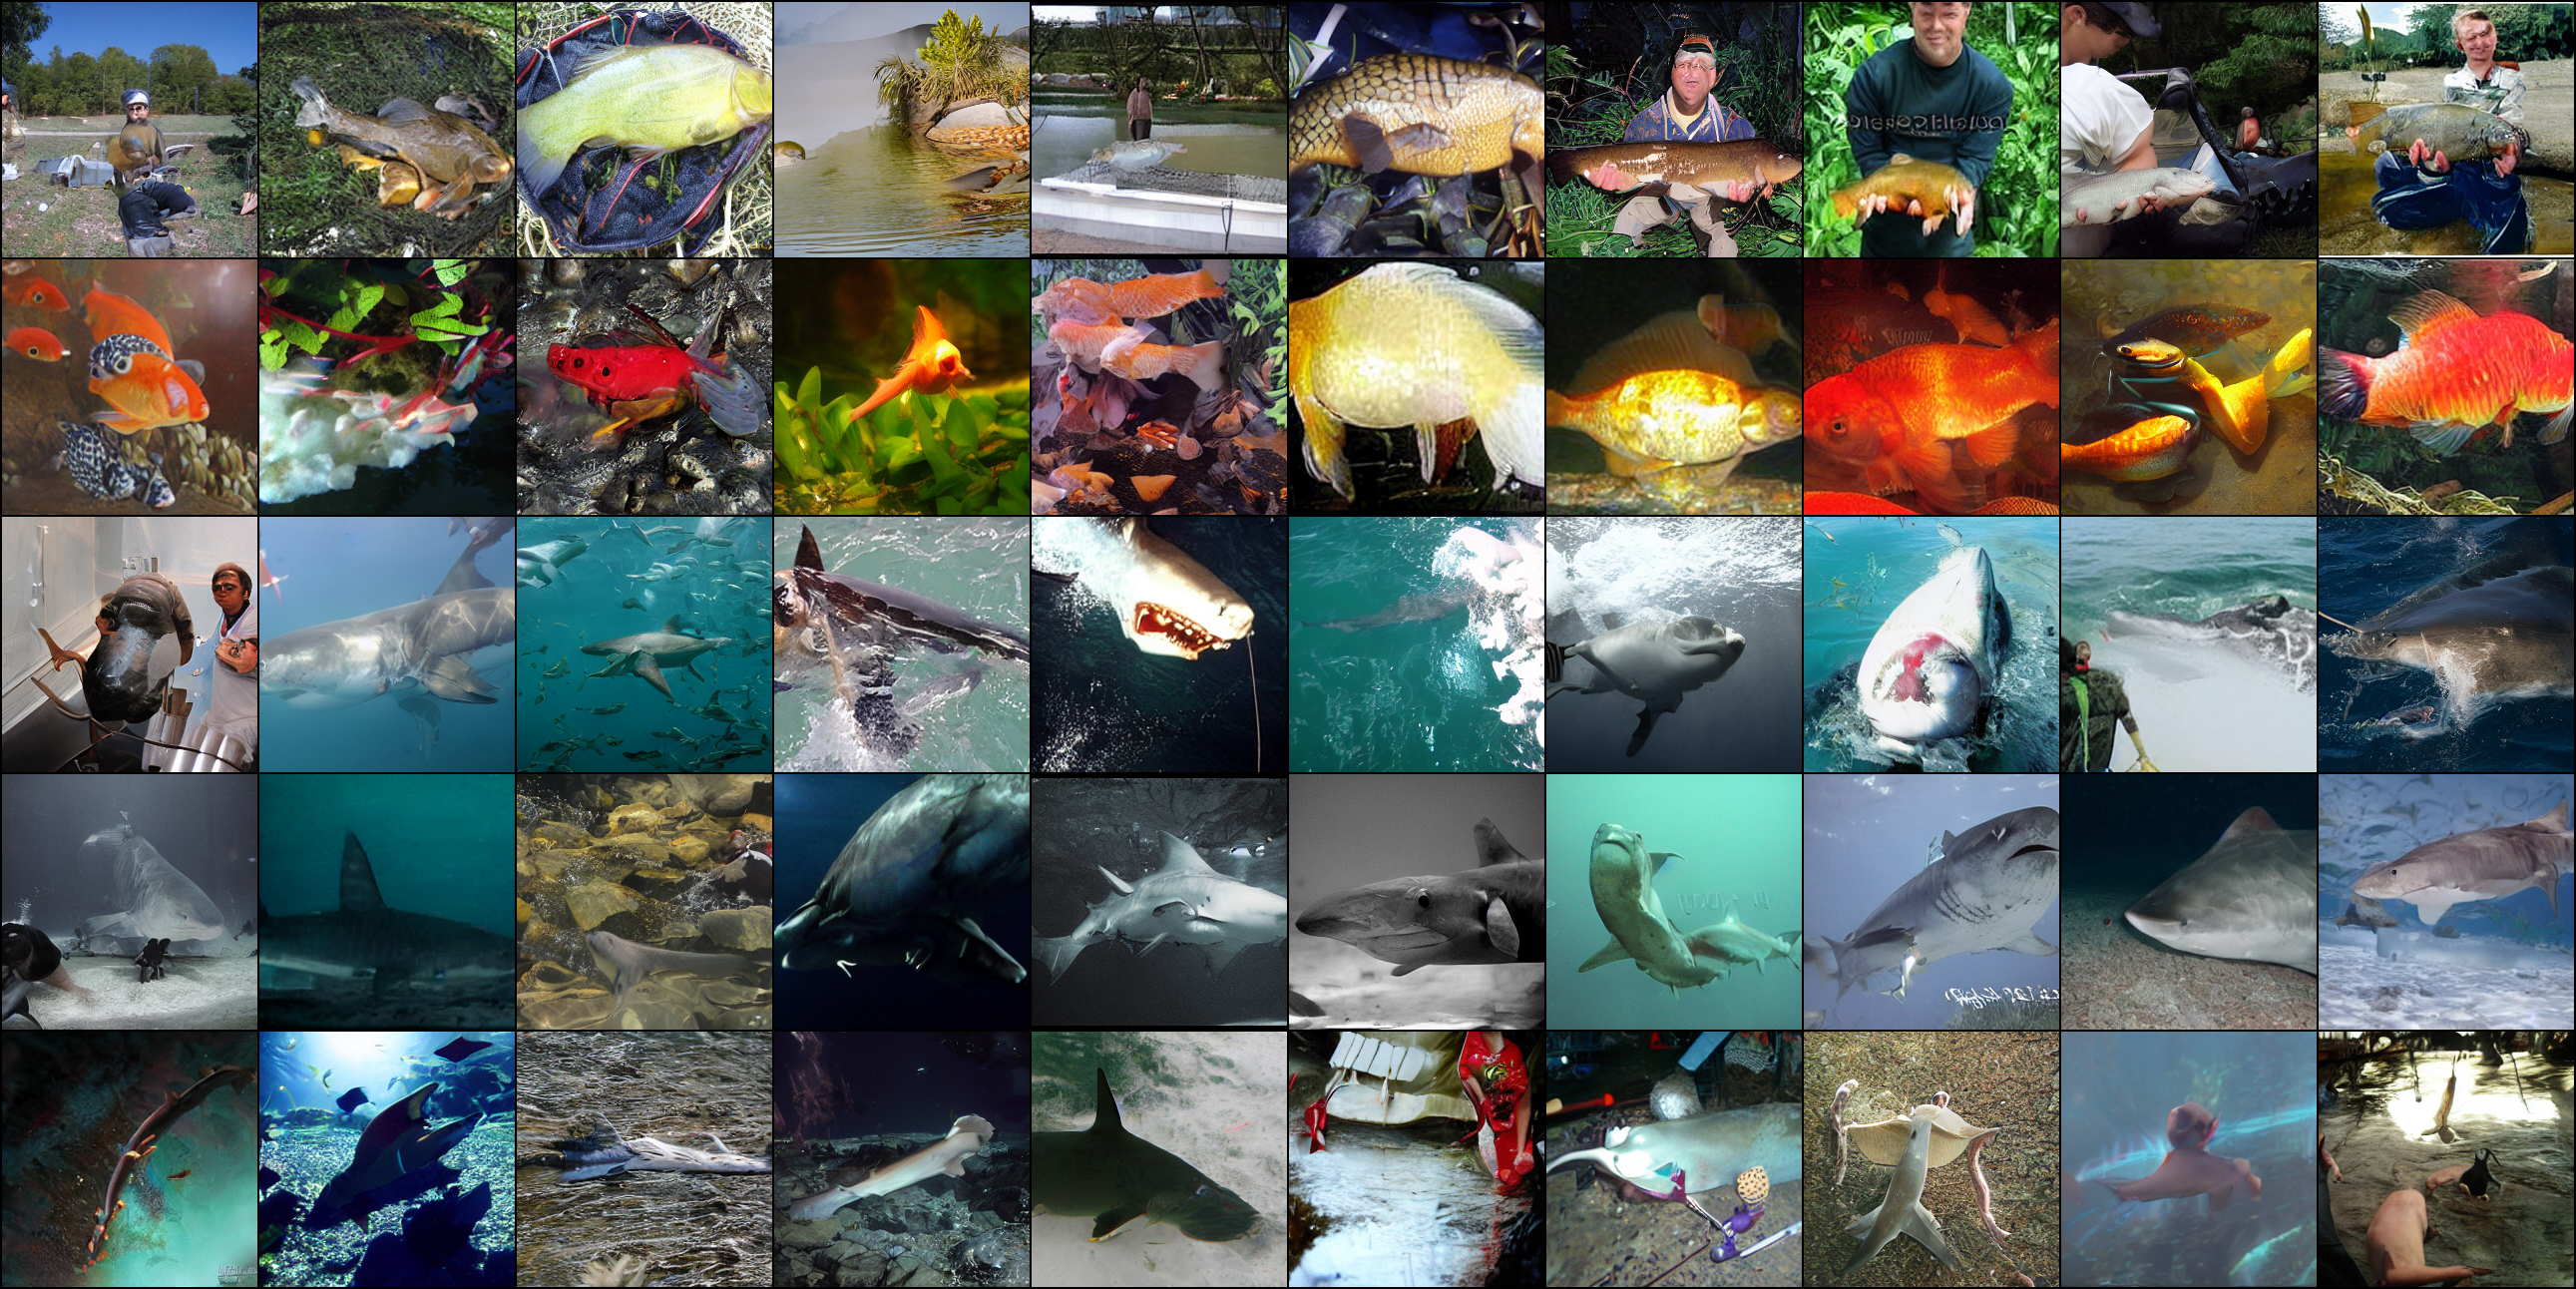}}
    \caption{Generation Samples on CIFAR-10, Celeb-A, MS-COCO and ImageNet}
    \label{fig:enter-label}
\end{figure*}
